# Supplementary material for: Stochastic diffusion using mean-field limits to approximate master equations
Source: arXiv:2408.07755 ancillary file (2024-08-14)
Supplement: Supplementary file 1 [file LHD24_meanFLAME_supplement.pdf]

# Supplemental appendix of "Stochastic diffusion using mean-field limits to approximate master equations"

Laurent Hébert-Dufresne, Matthew M. Kling, Samuel F. Rosenblatt, Stephanie N. Miller, P. Alexander Burnham, Nicholas W. Landry, Nicholas J. Gotelli, Brian J. McGill

August 14, 2024

**Abstract.** This appendix provides the mean-FLAME equations for our more complicated case studies.

In all of what follows, the coupling around the mean-field limit is assumed to equal a truncated Poisson with a time-varying average:

$$\rho\left[x, y(t)\right] = \frac{y(t)^x e^{-y(t)}}{x!}\left(1 - \frac{\Gamma(x-1, y(t))}{x!}\right)^{-1} \tag{1}$$

where $\Gamma(a, b)$ is the upper incomplete gamma function and renormalizes $\rho$ following truncation below the mean-field limit.

## 1 Lotka-Volterra predator-prey dynamics

We denote $n_F$ the number of prey fish $n_F$ and $n_S$ the number of predator sharks. Mean-field limits start at $n_F = n_{cF}$ and $n_S = n_{cS}$. The general master equation of a Lotka-Volterra predator-prey system can be written like so for $n_F < n_{cF}$ and $n_S < n_{cS}$:

$$\begin{aligned}\frac{d}{dt}P_{n_F,n_S}(t) = &-\mu n_F(K_F - n_F)P_{n_F,n_S}(t) - \nu n_S P_{n_F,n_S}(t) - \beta n_F n_S P_{n_F,n_S}(t) + \mu(n_F-1)(K-n_F+1)P_{n_F-1,n_S}(t) \\ &+ \nu(n_S+1)P_{n_F,n_S+1}(t) + \beta(n_F+1)(n_S-1)P_{n_F+1,n_S-1}(t)\ .\end{aligned} \tag{2}$$

For large number of preys and a small number of predator, the system is eventually coupled to a mean-field limit. We write the following equations close to the limit in $n_F$ but with $n_S < n_{cS} - 1$:

$$\begin{aligned}\frac{d}{dt}P_{n_{cF}-1,n_S}(t) = &-\mu(n_{cF}-1)(K_F - n_{cF}+1)P_{n_{cF}-1,n_S}(t) - \nu n_S P_{n_{cF}-1,n_S}(t) - \beta(n_{cF}-1)n_S P_{n_{cF}-1,n_S}(t) \\ &+ \mu(n_{cF}-2)(K_F - n_{cF}+2)P_{n_{cF}-2,n_S}(t) + \nu(n_S+1)P_{n_{cF}-1,n_S+1}(t) \\ &+ \beta n_{cF}(n_S-1)\rho\left[n_{cF}, F_{n_S-1}(t)\right]P_{n_{cF},n_S-1}(t)\ .\end{aligned} \tag{3}$$

Then, close to the limit in $n_S$ but with $n_F < n_{cS} - 1$, we have:

$$\begin{aligned}\frac{d}{dt}P_{n_F,n_{cS}-1}(t) = &-\mu n_F(K_F - n_F)P_{n_F,n_S}(t) - \nu(n_{cS}-1)P_{n_F,n_{cS}-1}(t) - \beta n_F(n_{cS}-1)P_{n_F,n_{cS}-1}(t) \\ &+ \mu(n_F-1)(K_F-n_F+1)P_{n_F-1,n_S}(t) + \nu n_{cS}\rho\left[n_{cS}, S_{n_F}(t)\right]P_{n_F,n_{cS}}(t) \\ &+ \beta(n_F+1)(n_{cS}-2)P_{n_F+1,n_{cS}-2}(t)\ .\end{aligned} \tag{4}$$

We also need to consider the case where both $n_F$ and $n_S$ are next to their mean-field limit:

$$\begin{aligned}\frac{d}{dt}P_{n_{cF}-1,n_{cS}-1}(t) = &-\mu(n_{cF}-1)(K_F-n_{cF}+1)P_{n_{cF}-1,n_{cS}}(t) - \nu(n_{cS}-1)P_{n_{cF},n_{cS}-1}(t) \\ &+ \mu(n_{cF}-2)(K_F-n_{cF}+2)P_{n_{cF}-2,n_{cS}-1}(t) + \nu n_{cS}\rho\left[n_{cS}, S_{n_F}(t)\right]P_{n_{cF}-1,n_{cS}}(t) \\ &+ \beta n_{cF}(n_{cS}-2)\rho\left[n_{cF}, F_{n_{cS}-1}(t)\right]P_{n_{cF},n_{cS}-2}(t) - \beta(n_{cF}-1)(n_{cS}-1)P_{n_{cF}-1,n_{cS}-1}(t)\ .\end{aligned} \tag{5}$$

As for the mean-field limits themselves, we first write the equation that governs the occupation number of the corresponding mean-field limit in the number of prey with a known number of predator $n_S < n_{cS} - 1$,

$$\frac{d}{dt}P_{n_{cF},n_S}(t) = -\nu n_S P_{n_{cF},n_S}(t) - \beta F_{n_S}(t) n_S P_{n_{cF},n_S}(t) + \mu(n_{cF}-1)(K_F - n_{cF}+1)P_{n_{cF}-1,n_S}(t) \\ + \nu(n_S+1)P_{n_{cF}-1,n_S+1}(t) + \beta F_{n_S-1}(t)(n_S-1)\{1-\rho\left[n_{cF},F_{n_S-1}(t)\right]\}P_{n_{cF},n_S-1}(t)\ , \tag{6}$$

and similarly for the mean-field in the number of predator with a known number of fish $n_F < n_{cF} - 1$,

$$\frac{d}{dt}P_{n_F,n_{cS}}(t) = -\mu n_F(K_F - n_F)P_{n_F,n_{cS}}(t) - \nu n_{cS}\rho\left[n_{cS},S_{n_F}(t)\right]P_{n_F,n_{cS}}(t) + \beta(n_F+1)S_{n_F+1}(t)P_{n_F+1,n_{cS}}(t) \tag{7} \\ + \beta(n_F+1)(n_{cS}-1)P_{n_F+1,n_{cS}-1}(t) + -\beta n_F S_{n_F}(t)P_{n_F,n_{cS}}(t) + \mu(n_F-1)(K_F-n_F+1)P_{n_F-1,n_S}(t)\ ,$$

These last two equations are slightly different next to mean-field limits. When $n_S = n_{cS} - 1$, we write

$$\frac{d}{dt}P_{n_{cF},n_{cS}-1}(t) = -\nu(n_{cS}-1)P_{n_{cF},n_{cS}-1}(t) - \beta(n_{cS}-1)\{\left[1-\rho\left[n_{cF},F_{n_{cS}-1}(t)\right]\right]F_{n_{cS}-1}(t) \\ + \rho\left[n_{cF},F_{n_{cS}-1}(t)\right]\}P_{n_{cF},n_{cS}-1}(t) + \mu(n_{cF}-1)(K_F-n_{cF}+1)P_{n_{cF}-1,n_S}(t) \\ + \nu(n_S+1)P_{n_{cF}-1,n_S+1}(t) + \beta F_{n_S-1}(t)(n_S-1)\{1-\rho\left[n_{cF},F_{n_S-1}(t)\right]\}P_{n_{cF},n_S-1}(t)\ , \tag{8}$$

or when $n_F = n_{cF} - 1$,

$$\frac{d}{dt}P_{n_{cF}-1,n_{cS}}(t) = -\mu(n_{cF}-1)(K_F-n_{cF}+1)P_{n_{cF}-1,n_{cS}}(t) - \nu n_{cS}\rho\left[n_{cS},S_{n_{cF}-1}(t)\right]P_{n_{cF}-1,n_{cS}}(t) \\ - \beta(n_{cF}-1)S_{n_{cF}-1}(t)P_{n_{cF}-1,n_{cS}}(t) + \mu(n_{cF}-2)(K_F-n_{cF}+2)P_{n_{cF}-2,n_S}(t) \\ + \beta n_{cF}\rho\left[n_{cF},F_{n_{cS}-1}(t)\right](n_{cS}-1)P_{n_{cF},n_{cS}-1}(t) + \beta n_{cF}\rho\left[n_{cF},F_{n_{cS}}(t)\right]S_{n_{cF}}(t)P_{n_{cF},n_{cS}}(t)\ , \tag{9}$$

And our final occupation number then track the probability of finding the system in a double mean-field regime

$$\frac{d}{dt}P_{n_{cF},n_{cS}}(t) = -\nu n_{cS}\rho\left[n_{cS},S_{n_{cF}}(t)\right]P_{n_{cF},n_{cS}}(t) - \beta n_{cF}\rho\left[n_{cF},F_{n_{cS}}(t)\right]S_{n_{cF}}(t)P_{n_{cF},n_{cS}}(t) \tag{10} \\ + \beta(n_{cF}-1)F_{n_{cS}-1}(t)\{1-\rho\left[n_{cF},F_{n_{cS}-1}(t)\right]\}P_{n_{cF},n_{cS}-1}(t) + \mu(n_{cF}-1)(K_F-n_{cF}+1)P_{n_{cF}-1,n_S}(t)\ .$$

Lastly, we need to track all the mean-field quantities with simpler mean-field equations. First, the number of prey with small number of predator $n_S < n_{cS}$:

$$\frac{d}{dt}F_{n_S}(t) = \mu F_{n_S}(t)(K - F_{n_S}(t)) - \beta n_S F_{n_S}(t)\ ; \tag{11}$$

second, the number of predators with small number of preys $n_F < n_{cF}$:

$$\frac{d}{dt}S_{n_F}(t) = \beta n_F S_{n_F}(t) - \nu S_{n_F}(t)\ ; \tag{12}$$

and lastly, the double mean-field regime:

$$\frac{d}{dt}F_{n_{cS}}(t) = \mu F_{n_{cS}}(t)(K - F_{n_{cS}}(t)) - \beta S_{n_{cF}}(t)F_{n_{cS}}(t) \\ \frac{d}{dt}S_{n_{cF}}(t) = \beta F_{n_{cS}}(t)S_{n_{cF}}(t) - \nu S_{n_{cF}}(t)\ ; \tag{13}$$

## 2 Metapopulation Susceptible-Infectious-Recovered-Susceptible epidemic dynamics

The model is now embedded in space over a metapopulation structure of populations of size $N(x, y)$ over discrete locations $(x, y)$. Let $i$ and $r$ be the number of infectious and recovered individuals in a population, and $N$ be its total population. Of course, these quantities can vary over time and space, but we omit the $(x, y)$ indices for simplicity. With a transmission rate $\beta$ within populations, an average coupling $\theta$ between populations, a recovery rate $\alpha$ and a waning immunity rate $\gamma$, we write a general master equation for numbers $i$ and $r$ not at or next to their mean-field limit (i.e., $i < n_i$ and $r < n_r$)

$$\begin{aligned}\frac{d}{dt}P_{i,r}(t) =& -(\beta i + \theta)(N - i - r)P_{i,r}(t) - \alpha i P_{i,r}(t) - \gamma r P_{i,r}(t) \\ &+ (\beta(i-1) + \theta)(N - i - r + 1)P_{i-1,r}(t) + \alpha(i+1)P_{i+1,r-1}(t) + \gamma(r+1)P_{i,r+1}(t) \; . \end{aligned} \tag{14}$$

When the infectious population is next to its mean-field limit, $i = n_i - 1$, we write:

$$\begin{aligned}\frac{d}{dt}P_{n_i-1,r}(t) =& -(\beta(n_i-1) + \theta)(N - n_i + 1 - r)P_{n_i-1,r}(t) - \alpha(n_i-1)P_{n_i-1,r}(t) - \gamma r P_{n_i-1,r}(t) \\ &+ (\beta(n_i-2) + \theta)(N - n_i - r + 2)P_{n_i-2,r}(t) + \alpha n_i \rho\left[n_i, I_{r-1}(t)\right] P_{n_i,r-1}(t) + \gamma(r+1)P_{n_i-1,r+1}(t) \; . \end{aligned} \tag{15}$$

Likewise, when the recovered population is next to its mean-field limit, $r = n_r - 1$, we write:

$$\begin{aligned}\frac{d}{dt}P_{i,n_r-1}(t) =& -(\beta i + \theta)(N - i - n_r + 1)P_{i,n_r-1}(t) - \alpha i P_{i,r}(t) - \gamma(n_r-1)P_{i,n_r-1}(t) \\ &+ (\beta(i-1) + \theta)(N - i - n_r + 2)P_{i-1,n_r-1}(t) + \alpha(i+1)P_{i+1,n_r-1}(t) + \gamma n_r \rho\left[n_r, R_i(t)\right] P_{i,n_r}(t) \; . \end{aligned} \tag{16}$$

When $i = n_i - 1$ and $r = n_r - 1$, we combine the last two to obtain

$$\begin{aligned}\frac{d}{dt}P_{n_i-1,n_r-1}(t) =& -(\beta(n_i-1) + \theta)(N - n_i - n_r + 2)P_{n_i-1,n_r-1}(t) - \alpha(n_i-1)P_{n_i-1,n_e-1}(t) - \gamma(n_r-1)P_{n_i-1,n_r-1}(t) \\ &+ (\beta(n_i-2) + \theta)(N - n_i - n_r + 3)P_{n_i-2,n_r-1}(t) + \alpha n_i \rho\left[n_i, I_{n_r-1}(t)\right] P_{n_i,n_r-2}(t) \\ &+ \gamma n_r \rho\left[n_r, R_{n_i-1}(t)\right] P_{n_i-1,n_r}(t) \; . \end{aligned} \tag{17}$$

When $i$ is in its mean-field limit and $r < n_r - 1$, we write

$$\begin{aligned}\frac{d}{dt}P_{n_i,r}(t) =& (\beta(n_i-1) + \theta)(N - n_i - r + 1)P_{n_i-1,r}(t) + \gamma(r+1)P_{n_i,r+1}(t) - \gamma r P_{n_i,r}(t) \\ &- \alpha I_r(t)\{1 - \rho\left[n_i, I_r(t)\right]\}P_{n_i,r}(t) - \alpha n_i \rho\left[n_i, I_r(t)\right] P_{n_i,r}(t) + \alpha I_{r-1}(t)\{1 - \rho\left[n_i, I_{r-1}(t)\right]\}P_{n_i,r-1}(t) \; . \end{aligned} \tag{18}$$

When $i$ is in its mean-field limit and $r = n_r - 1$, we instead write

$$\begin{aligned}\frac{d}{dt}P_{n_i,n_r-1}(t) =& (\beta(n_i-1) + \theta)(N - n_i - n_r + 2)P_{n_i-1,n_r-1}(t) + \gamma n_r \rho\left[n_r, R_{n_i}(t)\right] P_{n_i,n_r}(t) - \gamma(n_r-1)P_{n_i,n_r-1}(t) \\ &- \alpha I_{n_r-1}(t)\{1 - \rho\left[n_i, I_{n_r-1}(t)\right]\}P_{n_i,n_r-1}(t) - \alpha n_i \rho\left[n_i, I_{n_r-1}(t)\right] P_{n_i,n_r-1}(t) \\ &+ \alpha I_{n_r-2}(t)\{1 - \rho\left[n_i, I_{n_r-2}(t)\right]\}P_{n_i,n_r-2}(t) \; . \end{aligned} \tag{19}$$

Likewise, when $r$ is in its mean-field limit and $i < n_i - 1$, we write

$$\begin{aligned}\frac{d}{dt}P_{i,n_r}(t) =& -(\beta i + \theta)(N - i - R_i(t))P_{i,n_r}(t) - \alpha i P_{i,n_r}(t) - \gamma n_r \rho\left[n_r, R_i(t)\right] P_{i,n_r}(t) \\ &+ (\beta(i-1) + \theta)(N - i - R_{i-1}(t) + 1)P_{i-1,n_r}(t) + \alpha(i+1)P_{i+1,n_r-1}(t) + \alpha(i+1)P_{i+1,n_r}(t) \; . \end{aligned} \tag{20}$$

And when $r$ is in its mean-field limit and $i = n_i - 1$, we instead write

$$\frac{d}{dt}P_{n_i-1,n_r}(t) = -\left(\beta(n_i-1)+\theta\right)(N-n_i-R_i(t)+1)P_{n_i-1,n_r}(t) - \alpha(n_i-1)P_{n_i-1,n_r}(t) - \gamma n_r\rho\left[n_r, R_{n_i-1}(t)\right]P_{n_i-1,n_r}(t)$$
$$+\left(\beta(n_i-2)+\theta\right)(N-n_i-R_{i-1}(t)+2)P_{n_i-2,n_r}(t) + \alpha n_i\rho\left[n_i, I_{n_r-1}(t)\right]P_{n_i,n_r-1}(t) + \alpha n_i\rho\left[n_i, I_{n_r}(t)\right]P_{n_i,n_r}(t)\ . \quad (21)$$

And finally, the occupation number of the double mean-field limit can be tracked by

$$\frac{d}{dt}P_{n_i,n_r}(t) = -\alpha n_i\rho\left[n_i, I_{n_r}(t)\right]P_{n_i,n_r}(t) - \gamma n_r\rho\left[n_r, R_{n_i}(t)\right]P_{n_i,n_r}(t)$$
$$+\left(\beta(n_i-1)+\theta\right)(N-n_i-R_{n_i-1}(t)+1)P_{n_i-1,n_r}(t) + \alpha I_{n_r-1}(t)\{1-\rho\left[n_i, I_{n_r-1}(t)\right]\}P_{n_i,n_r-1}(t)\ . \quad (22)$$

The previous equations track the probability distribution of the system over all of its possible states but requires a few mean-field quantities to be a closed system. First, the coupling between populations $\theta$ is calculated like so:

$$\theta^{(x,y)} = \lambda\beta\sum_{j\in\mathcal{N}_{(x,y)}}\left\{\sum_{i,r} iP^{(j)}_{i,r}(t) + \sum_r I_r(t)P^{(j)}_{I_r(t),r}(t) + I_{R(t)}(t)P^{(j)}_{I_R(t),R_I(t)}\right\}\ , \quad (23)$$

which is proportional to the transmission rate $\beta$, the coupling rate $\lambda$, and to the average number of infectious individuals in populations $j$ that are neighboring the $(x,y)$ population considered.

Second, we also then need to track a suite of mean-field quantities: the number of infectious individuals with small number of recovered $r < n_r$:

$$\frac{d}{dt}I_r(t) = (\beta I_r(t)+\theta)(N-I_r(t)-r) - \alpha I_r(t)\ ; \quad (24)$$

for the number of recovered individuals with small number of infectious $i < n_i - 1$, we actually track recovery events using transitions in the master equation to avoid a constant influx of recoveries:

$$\frac{d}{dt}R_i(t) = \alpha(i+1)\left[P_{i+1,n_r-1}(t) + P_{i+1,n_r}(t)\right] - \gamma R_i(t)\ ; \quad (25)$$

and we do the same for $i = n_i - 1$:

$$\frac{d}{dt}R_{n_i-1}(t) = \alpha n_i\{\rho\left[n_i, I_{n_r}(t)\right]P_{n_i,n_r}(t) + \rho\left[n_i, I_{n_r-1}(t)\right]P_{n_i,n_r-1}(t)\} - \gamma R_i(t)\ ; \quad (26)$$

and lastly, the double mean-field regime does not have the same issue so we write:

$$\frac{d}{dt}I_{n_r}(t) = (\beta I_r(t)+\theta)(N-I_{n_r}(t)-R_{n_i}(t)) - \alpha I_{n_r}(t)$$
$$\frac{d}{dt}R_{n_i}(t) = \alpha I_{n_r}(t) - \gamma R_{n_i}(t)\ . \quad (27)$$

All of the equations above are repeated for every population in the metapopulation system, with the key difference being their different total size $N$ as well as their set of neighbors $\mathcal{N}$ in Eq. (23).

## 3 Species dispersal model with complex life cycles

In this final model, we consider a four-stage life cycle for the tree species: (i) Seeds ($s$), (ii) seedlings or small greens ($g$), (iii) saplings or young trees ($y$), and (iv) adult trees ($a$). Every population also has two quantities only described by their mean-field: the number of seeds $S_{y,a}(t)$ and seedlings or small greens $G_{y,a}(t)$. We then use mean-FLAME to describe the number of saplings or young trees.

The life cycle is a simple loop where seeds die at rate $\nu_s$ or grow into greens at rate $\mu_s$ , which die at rate $\nu_g$ or grow into young trees at rate $\mu_g$, which die at rate $\nu_y$ and compete for resources to grow into adult trees at a rate equal to $\mu_y$ times the square root of the number of young trees times the difference between the carrying capacity $K$ and the current population. Adult trees produce seeds at a large rate $\mu_a$ both locally and at neighboring sites through seed dispersal. Any of these parameters can vary through space and time, although our case study only varies $K(x, y, t)$. We omit the spatial and temporal dependency and simply write $K$ for clarity as the notation is involved enough as it is.

Given all of this, we can write a general master equation for numbers $y$ and $a$ not at or next to their mean-field limit (i.e., $y < n_y - 1$ and $a < n_a - 1$):

$$\begin{aligned}\frac{d}{dt}P_{y,a}(t) =& \nu_y(y+1)P_{y+1,a}(t) - \nu_y y P_{y,a}(t) + \mu_g G_{y-1,a}(t)P_{y-1,a}(t) - \mu_g G_{y,a}(t)P_{y,a}(t) \\ &+ \mu_y\sqrt{y+1}(K-a+1)P_{y+1,a-1}(t) - \mu_y\sqrt{y}(K-a)P_{y,a}(t) + \nu_a(a+1)P_{y,a+1}(t) - \nu_a a P_{y,a}(t)\end{aligned} \quad (28)$$

When the young tree population is next to its mean-field limit, $y = n_y - 1$, we write:

$$\begin{aligned}\frac{d}{dt}P_{n_y-1,a}(t) =& \nu_y n_y \rho\left[n_y, Y_a(t)\right] P_{n_y,a}(t) - \nu_y(n_y-1)P_{n_y-1,a}(t) + \mu_g G_{n_y-2,a}(t)P_{n_y-2,a}(t) - \mu_g G_{n_y-1,a}(t)P_{n_y-1,a}(t) \\ &+ \mu_y\sqrt{n_y}(K-a)\rho\left[n_y, Y_{a-1}(t)\right] P_{n_y,a-1}(t) - \mu_y\sqrt{n_y-1}(K-a)P_{n_y-1,a}(t) \\ &+ \nu_a(a+1)P_{n_y-1,a+1}(t) - \nu_a a P_{n_y-1,a}(t)\end{aligned} \quad (29)$$

Likewise, when the adult tree population is next to its mean-field limit, $a = n_a - 1$, we write:

$$\begin{aligned}\frac{d}{dt}P_{y,n_a-1}(t) =& \nu_y(y+1)P_{y+1,n_a-1}(t) - \nu_y y P_{y,n_a-1}(t) + \mu_g G_{y-1,n_a-1}(t)P_{y-1,n_a-1}(t) - \mu_g G_{y,n_a-1}(t)P_{y,n_a-1}(t) \\ &+ \mu_y\sqrt{y+1}(K-n_a+1)P_{y+1,n_a-1}(t) - \mu_y\sqrt{y}(K-n_a+1)P_{y,n_a-1}(t) \\ &+ \nu_a n_a \rho\left[n_a, A_y(t)\right] P_{y,n_a}(t) - \nu_a(n_a-1)P_{y,n_a-1}(t) \ ,\end{aligned} \quad (30)$$

and we combine the last two equations when both $y = n_y - 1$ and $a = n_a - 1$,

$$\begin{aligned}\frac{d}{dt}P_{n_y-1,n_a-1}(t) =& \nu_y n_y \rho\left[n_y, Y_{n_a-1}(t)\right] P_{n_y,n_a-1}(t) - \nu_y(n_y-1)P_{n_y-1,n_a-1}(t) + \mu_g G_{n_y-2,n_a-1}(t)P_{n_y-2,n_a-1}(t) \\ &- \mu_g G_{n_y-1,n_a-1}(t)P_{n_y-1,n_a-1}(t) + \mu_y\sqrt{n_y}(K-n_a+1)\rho\left[n_y, Y_{n_a-1}(t)\right] P_{n_y,n_a-1}(t) \\ &- \mu_y\sqrt{n_y-1}(K-n_a+1)P_{n_y-1,n_a-1}(t) + \nu_a n_a \rho\left[n_a, A_{n_y-1}(t)\right] P_{n_y-1,n_a}(t) - \nu_a(n_a-1)P_{n_y-1,n_a-1}(t) \ ,\end{aligned} \quad (31)$$

Beyond these master equations state, when $y$ is in its mean-field limit and $a < n_a - 1$ we write

$$\begin{aligned}\frac{d}{dt}P_{n_y,a}(t) =& -\nu_y n_y \rho\left[n_y, Y_a(t)\right] P_{n_y,a}(t) + \mu_g G_{n_y-1,a}(t)P_{n_y-1,a}(t) - \mu_y\sqrt{n_y}(K-a)\rho\left[n_y, Y_a(t)\right] P_{n_y,a}(t) \\ &- \mu_y\sqrt{Y_a(t)}(K-a)(1-\rho\left[n_y, Y_a(t)\right])P_{n_y,a}(t) - \nu_a a P_{n_y,a}(t) \\ &+ \mu_y\sqrt{Y_{a-1}(t)}(K-a+1)(1-\rho\left[n_y, Y_{a-1}(t)\right])P_{n_y,a-1}(t) + \nu_a(a+1)P_{n_y,a+1}(t) \ .\end{aligned} \quad (32)$$

In the mean-field limit for $y$ with $a = n_a - 1$, we instead use

$$\begin{aligned}\frac{d}{dt}P_{n_y,n_a-1}(t) =& -\nu_y n_y \rho\left[n_y, Y_{n_a-1}(t)\right] P_{n_y,n_a-1}(t) + \mu_g G_{n_y-1,n_a-1}(t) P_{n_y-1,n_a-1}(t) - \nu_a (n_a-1) P_{n_y,n_a-1}(t) \\ & - \mu_y \sqrt{Y_{n_a-1}(t)}(K - n_a + 1)(1 - \rho\left[n_y, Y_{n_a-1}(t)\right]) P_{n_y,n_a-1}(t) - \mu_y \sqrt{n_y}(K - n_a + 1)\rho\left[n_y, Y_{n_a-1}(t)\right] P_{n_y,n_a-1}(t) \\ & + \mu_y \sqrt{Y_{n_a-2}(t)}(K - n_a + 2)(1 - \rho\left[n_y, Y_{n_a-2}(t)\right]) P_{n_y,n_a-2}(t) + \nu_a n_a \rho\left[n_a, A_{n_y}(t)\right] P_{n_y,n_a}(t) \; . \end{aligned} \tag{33}$$

Conversely, when $a$ is in its mean-field limit and $y < n_y - 1$ we write

$$\begin{aligned}\frac{d}{dt}P_{y,n_a}(t) =& -\nu_y y P_{y,n_a}(t) - \mu_y \sqrt{y}(K - A_y(t)) P_{y,n_a}(t) + \mu_y \sqrt{y+1}(K - n_a + 1) P_{y+1,n_a-1}(t) \\ & - \nu_a a \rho\left[n_a, A_y(t)\right] P_{y,n_a}(t) + \mu_g G_{y-1,n_a}(t) P_{y-1,n_a}(t) - \mu_g G_{y,n_a}(t) P_{y,n_a}(t) \\ & + \mu_y \sqrt{y+1}(K - A_{y+1}(t)) P_{y+1,n_a}(t) + \nu_y (y+1) P_{y+1,n_a}(t) \; . \end{aligned} \tag{34}$$

In the mean-field limit for $a$ with $y = n_y - 1$, we instead use

$$\begin{aligned}\frac{d}{dt}P_{n_y-1,n_a}(t) =& -\nu_y (n_y-1) P_{n_y-1,n_a}(t) - \mu_y \sqrt{n_y-1}(K - A_{n_y-1}(t)) P_{n_y-1,n_a}(t) + \mu_y \sqrt{n_y}(K - n_a + 1)\rho\left[n_y, Y_{n_a}(t)\right] P_{n_y,n_a}(t) \\ & - \nu_a a \rho\left[n_a, A_{n_y-1}(t)\right] P_{n_y-1,n_a}(t) + \mu_g G_{n_y-2,n_a}(t) P_{n_y-2,n_a}(t) - \mu_g G_{n_y-1,n_a}(t) P_{n_y-1,n_a}(t) \\ & + \mu_y \sqrt{n_y}\rho\left[n_y, Y_{n_a}(t)\right](K - A_{n_y}(t)) P_{n_y,n_a}(t) + \nu_y n_y \rho\left[n_y, Y_{n_a}(t)\right] P_{n_y,n_a}(t) \; . \end{aligned} \tag{35}$$

Finally, we write the equation for the double mean-field regime,

$$\begin{aligned}\frac{d}{dt}P_{n_y,n_a}(t) =& -\nu_y n_y \rho\left[n_y, Y_{n_a}(t)\right] P_{n_y,n_a}(t) P_{n_y,n_a}(t) - \mu_y \sqrt{n_y}(K - A_{n_y}(t))\rho\left[n_y, Y_{n_a}(t)\right] P_{n_y,n_a}(t) - \nu_y n_y \rho\left[n_y, Y_{n_a}(t)\right] P_{n_y,n_a}(t) \\ & + \mu_y \sqrt{Y_{n_a-1}(t)}(K - n_a + 1)\{1 - \rho\left[n_y, Y_{n_a-1}(t)\right]\} P_{n_y,n_a-1}(t) + \mu_g G_{n_y-1,n_a}(t) P_{n_y-1,n_a}(t) \; . \end{aligned} \tag{36}$$

This completes the system of equation to track the distribution probability over all possible system states at a given spatial site. We can close the system with a rather large set of mean-field equations for each possible site. First, we need an equation for the number of seeds at every location:

$$\frac{d}{dt}S_{y,a}(t) = \theta + \mu_a a P_{y,a}(t) - (\nu_s + \mu_s) S_{y,a}(t) \tag{37}$$

where $\theta$ is again our mean-field coupling to other location. We use a similar equation for systems in their mean-field limit and replace the $a$ factor with their mean-field quantity. For this model, the spatial coupling $\theta$ is a function of seed dispersal from neighbors around the local site $(x, y)$:

$$\theta^{(x,y)} = \lambda \mu_a \sum_{j \in \mathcal{N}_{(x,y)}} \left\{ \sum_{y,a} a P^{(j)}_{y,a}(t) + \sum_{r} A_y(t) P^{(j)}_{y,n_a}(t) \right\} , \tag{38}$$

where the first sum is over all states whose number of adult trees is outside of the mean-field limit, and the second sum is for all states in the mean-field limit for adult trees. We also note that, in this case, we use $\lambda = 1$ for simplicity.

Second, we write an equation for the number of seedlings (or greens $G$), at every location for every possible state:

$$\frac{d}{dt}G_{y,a}(t) = \mu_s S_{y,a}(t) - (\nu_g + \mu_g) G_{y,a}(t) \; . \tag{39}$$

Third, like in the previous models, we write a series of mean-field equations corresponding to possible states for young and adult trees. When young trees are in their mean-field limit and adult trees in $a < n_a - 1$, we write

$$\frac{d}{dt}Y_a(t) = \mu_g G_{y,a}(t) - \nu_y Y_a(t) + \mu_y \sqrt{Y_a(t)}(K - a) \ . \tag{40}$$

Conversely, when adult trees are in their mean-field limit and young trees in $y < n_y - 1$, we write

$$\frac{d}{dt}A_y(t) = \mu_y \sqrt{y}(K - A_y(t)) - \nu_a A_y(t) \ . \tag{41}$$

And, in the double mean-field regime, we find a combination of the two previous equations,

$$\begin{aligned} \frac{d}{dt}Y_{n_a}(t) &= \mu_g G_{n_y,n_a}(t) - \nu_y Y_{n_a}(t) - \mu_y \sqrt{Y_{n_a}(t)}(K - A_{n_y}(t)) \\ \frac{d}{dt}A_{n_y}(t) &= \mu_y \sqrt{Y_{n_a}(t)}(K - A_{n_y}(t)) - \nu_a A_{n_y}(t) \ . \end{aligned} \tag{42}$$

This last equation closes the mean-FLAME model for our four-stage life-cycle tree dispersal model.
